# Supplementary material for: Safe and Private Forward-Trading Platform for Transactive Microgrids
Source: arXiv:1910.12579 source file (2019-10-11)
Supplement: Supplementary file 1 [file appendix.tex]

\section{Appendix}

\subsection{Coin Shuffle}
\input{figs/mix.tex}

Ruffing \textit{et al.} proposed a mixing service named \textit{CoinShuffle}  which is completely decentralized. The only drawback is that the algorithm requires at least two trusted participants so that the result is completely anonymous.

Figure~\ref{fig:mix} shows the procedure of CoinShuffle. CoinShuffle was initially created as a mixing service for Bitcoin, but it can be extended to support other distributed ledger platforms. The only requirement is that the ledger should support a transaction with multiple input and multiple output accounts. For example, this can be done via an smart contract on the Ethereum. This algorithm is done in 3 phases:
    \begin{description}
        \item[Phase 0:] The members of group $G$ decide on an order of members ($P_1, P_2, P_3, \cdots , P_n$) for message exchange and encryption. In \platform, this is  done via the smart contract. Further, each participant creates a new account on the ledger ($P_1^\prime, P_2^\prime, P_3^\prime, \cdots, P_n^\prime)$.
        \item[Phase 1:] Each member of $G$ creates an asymmetric encryption-decryption key pair ($E_{P_i}$ and $D_{P_i}$) and broadcast the signed public key to others.
        \item[Phase 2:] First member of the encryption order $P_1$ creates an empty list $T$. It encrypts its target account's address with others' public key in reverse order ($enc(E_{P_2}, enc(E_{P_3}, enc(\cdots,\allowbreak enc(E_{P_n}, P_1^\prime))))$), adds it to $T$ and send the list to $P_2$. When each participant $P_i$ receives $T$ from the previous one, it decrypts all elements to get an encrypted message for the next participant, encrypts its target account's address with all of the next participants' public keys, adds the encrypted message to $T$, and shuffles the list. After that, it will send $T$ to the next participant $P_{i+1}$. Finally, $P_n$ has a shuffled list of target accounts that we can use to transfer funds to.
        \item[Phase 3:] $P_n$ creates a transaction with all of $P_i$s' accounts as input and $T$ as the output. All $P_i$s need to sign the contract to ensure its integrity (e.g., every participant's anonymous account is present in the transaction). With that, the transaction will be executed and the assets are mixed in the target accounts.
\end{description}
